# Supplementary material for: Feedback Coding for Active Learning
Source: arXiv:2103.00654 source file (2021-02-28)
Supplement: Supplementary file 1 [file table_LR_supp.tex]

\begin{small}
\begin{tabular}{|S[table-format=2.3]|S[table-format=2.3]|S[table-format=2.3]|S[table-format=2.3]|S[table-format=2.3]|S[table-format=2.3]|S[table-format=2.3]|}
\hline
{} & {APM-LR} & {Uncertainty} & {BALD} & {InfoGain} & {Random} & {MaxVar} \\  
\hline
{\emph{vehicle-full}} & 0.022 & 0.019 & 0.021 & 0.022 & 0.020 & 0.022 \\  
\hline
{\emph{vehicle-cars}} & 0.025 & 0.023 & 0.025 & 0.026 & 0.024 & 0.026 \\  
\hline
{\emph{vehicle-transport}} & 0.021 & 0.020 & 0.022 & 0.022 & 0.021 & 0.022 \\  
\hline
{\emph{letterDP}} & 0.025 & 0.024 & 0.026 & 0.027 & 0.024 & 0.026 \\  
\hline
{\emph{letterEF}} & 0.022 & 0.023 & 0.023 & 0.026 & 0.023 & 0.024 \\  
\hline
{\emph{letterIJ}} & 0.023 & 0.022 & 0.024 & 0.025 & 0.023 & 0.024 \\  
\hline
{\emph{letterMN}} & 0.028 & 0.026 & 0.028 & 0.030 & 0.026 & 0.029 \\  
\hline
{\emph{letterUV}} & 0.021 & 0.021 & 0.021 & 0.024 & 0.021 & 0.022 \\  
\hline
{\emph{letterVY}} & 0.022 & 0.021 & 0.023 & 0.025 & 0.021 & 0.023 \\  
\hline
{\emph{austra}} & 0.025 & 0.023 & 0.025 & 0.025 & 0.023 & 0.025 \\  
\hline
{\emph{wdbc}} & 0.026 & 0.023 & 0.025 & 0.025 & 0.022 & 0.024 \\  
\hline
{\emph{clouds}} & 0.017 & 0.018 & 0.019 & 0.021 & 0.018 & 0.020 \\  
\hline
{\emph{cross}} & 0.020 & 0.020 & 0.022 & 0.023 & 0.021 & 0.023 \\  
\hline
{\emph{horseshoe}} & 0.016 & 0.016 & 0.017 & 0.018 & 0.016 & 0.016 \\  
\hline
\end{tabular}
\end{small}
