# Supplementary material for: Feedback Coding for Active Learning
Source: arXiv:2103.00654 source file (2021-02-28)
Supplement: Supplementary file 2 [file table_common_supp.tex]

\begin{small}
\begin{tabular}{|S[table-format=2.3]|S[table-format=2.3]|S[table-format=2.3]|S[table-format=2.3]|S[table-format=2.3]|S[table-format=2.3]|S[table-format=2.3]|}
\hline
{} & {APM-LR} & {Uncertainty} & {BALD} & {InfoGain} & {Random} & {MaxVar} \\  
\hline
{\emph{vehicle-full}} & 10.110 & 4.559 & 10.139 & 9.750 & 7.490 & 18.086 \\  
\hline
{\emph{vehicle-cars}} & 5.444 & 4.435 & 5.628 & 5.502 & 3.303 & 4.586 \\  
\hline
{\emph{vehicle-transport}} & 9.632 & 5.836 & 9.310 & 9.109 & 11.236 & 21.087 \\  
\hline
{\emph{letterDP}} & 7.647 & 6.435 & 6.925 & 6.786 & 10.723 & 11.875 \\  
\hline
{\emph{letterEF}} & 6.889 & 5.725 & 6.343 & 6.187 & 11.325 & 10.776 \\  
\hline
{\emph{letterIJ}} & 7.391 & 5.746 & 6.945 & 6.737 & 10.043 & 9.871 \\  
\hline
{\emph{letterMN}} & 8.219 & 6.309 & 7.643 & 7.412 & 10.108 & 13.259 \\  
\hline
{\emph{letterUV}} & 8.051 & 6.578 & 7.164 & 7.101 & 10.768 & 12.607 \\  
\hline
{\emph{letterVY}} & 7.486 & 5.781 & 7.170 & 6.934 & 8.256 & 10.003 \\  
\hline
{\emph{austra}} & 12.538 & 6.475 & 12.029 & 11.672 & 8.571 & 13.605 \\  
\hline
{\emph{wdbc}} & 18.002 & 10.911 & 14.208 & 13.938 & 20.785 & 29.800 \\  
\hline
{\emph{clouds}} & 1.241 & 1.188 & 1.177 & 1.345 & 3.222 & 5.340 \\  
\hline
{\emph{cross}} & 1.405 & 2.438 & 1.498 & 1.564 & 3.157 & 4.474 \\  
\hline
{\emph{horseshoe}} & 1.012 & 0.925 & 0.880 & 0.948 & 0.817 & 1.224 \\  
\hline
\end{tabular}
\end{small}
